# Supplementary material for: Emergent Communication with Attention
Source: arXiv:2305.10920 source file (2023-05-18)
Supplement: Supplementary file 1 [file 99-appendix.tex]

\newpage
\appendix
\section*{Appendix}
\input{sections/appendices/experimental_setup.tex}

\begin{figure*}[t]
% ======
\begin{minipage}{.33\linewidth}
\centering
\subfloat[\small{One-hot (8, 2): \TrainAcc}]{\label{fig:add-onehot_8_2-train}\includegraphics[width=\figWidth]{data/main_results/onehot_8_2-train.png}}
\end{minipage}\hfill%
% ======
\begin{minipage}{.33\linewidth}
\centering
\subfloat[\small{One-hot (8, 2): \GenAcc}]{\label{fig:add-onehot_8_2-gen}\includegraphics[width=\figWidth]{data/main_results/onehot_8_2-eval.png}}
\end{minipage}\hfill%
% ======
\begin{minipage}{.33\linewidth}
\centering
\subfloat[\small{One-hot (8, 2): \TopSim}]{\label{fig:add-onehot_8_2-topsim}\includegraphics[width=\figWidth]{data/main_results/onehot_8_2-topsim.png}}
\end{minipage}\par\medskip % ============================================
% ======
\begin{minipage}{.33\linewidth}
\centering
\subfloat[\small{One-hot (4, 4): \TrainAcc}]{\label{fig:add-onehot_4_4-train}\includegraphics[width=\figWidth]{data/appendix_results/onehot_4_4-train.png}}
\end{minipage}\hfill%
% ======
\begin{minipage}{.33\linewidth}
\centering
\subfloat[\small{One-hot (4, 4): \GenAcc}]{\label{fig:add-onehot_4_4-gen}\includegraphics[width=\figWidth]{data/appendix_results/onehot_4_4-eval.png}}
\end{minipage}\hfill%
% ======
\begin{minipage}{.33\linewidth}
\centering
\subfloat[\small{One-hot (4, 4): \TopSim}]{\label{fig:add-onehot_4_4-topsim}\includegraphics[width=\figWidth]{data/appendix_results/onehot_4_4-topsim.png}}
\end{minipage}\par\medskip % ============================================
% ======
\begin{minipage}{.33\linewidth}
\centering
\subfloat[\small{One-hot (16, 2): \TrainAcc}]{\label{fig:add-onehot_16_2-train}\includegraphics[width=\figWidth]{data/appendix_results/onehot_16_2-train.png}}
\end{minipage}\hfill%
% ======
\begin{minipage}{.33\linewidth}
\centering
\subfloat[\small{One-hot (16, 2): \GenAcc}]{\label{fig:add-onehot_16_2-gen}\includegraphics[width=\figWidth]{data/appendix_results/onehot_16_2-eval.png}}
\end{minipage}\hfill%
% ======
\begin{minipage}{.33\linewidth}
\centering
\subfloat[\small{One-hot (16, 2): \TopSim}]{\label{fig:add-onehot_16_2-topsim}\includegraphics[width=\figWidth]{data/appendix_results/onehot_16_2-topsim.png}}
\end{minipage}\par\medskip % ============================================
\caption{The results of the one-hot game with different configurations. The color of the boxes indicates the base architecture of the agents (LSTM or Transformer) and the x-axis labels indicates whether \Speaker and \Listener use attention.}
\label{fig:add-results}
\end{figure*}

\newpage

\begin{figure*}[ht]
% ============================================
\begin{minipage}{.5\linewidth}
\centering
\subfloat[LSTM]{\label{fig:arch-lstm}\includegraphics[width=5.2cm]{data/attention_agents/LSTM.jpeg}}
\end{minipage}\hfill
% ======
\begin{minipage}{.5\linewidth}
\centering
\subfloat[Transformer]{\label{fig:arch-transformer}\includegraphics[width=5.2cm]{data/attention_agents/Transformer.jpeg}}
\end{minipage}%
% ============================================
\caption{The architecture of the LSTM and Transformer decoders used in this paper.}
\label{fig:arch}
\end{figure*}

\newpage

\begin{figure*}[ht]
% ======
\begin{minipage}{.33\linewidth}
\centering
\subfloat[\small{One-hot: \TrainAcc}]{\label{fig:concat-onehot-train}\includegraphics[width=\figWidth]{data/appendix_results/onehot_8_2-concat-train.png}}
\end{minipage}\hfill%
% ======
\begin{minipage}{.33\linewidth}
\centering
\subfloat[\small{One-hot: \GenAcc}]{\label{fig:concat-onehot-gen}\includegraphics[width=\figWidth]{data/appendix_results/onehot_8_2-concat-gen.png}}
\end{minipage}\hfill%
% ======
\begin{minipage}{.33\linewidth}
\centering
\subfloat[\small{One-hot: \TopSim}]{\label{fig:concat-onehot-topsim}\includegraphics[width=\figWidth]{data/appendix_results/onehot_8_2-concat-topsim.png}}
\end{minipage}\par\medskip % ============================================
\caption{The comparison of different types of baseline object encoders.}
\label{fig:concat-results}
\end{figure*}

\newpage

\input{sections/appendices/multi-head.tex}
